# Supplementary material for: Conformal Prediction Sets with Limited False Positives
Source: arXiv:2202.07650 source file (2022-02-15)
Supplement: Supplementary file 1 [file conditional.tex]

\section{Calibration-conditional  False Positive Control}
\label{app:conditional}
