# Supplementary material for: Conformal Prediction Sets with Limited False Positives
Source: arXiv:2202.07650 source file (2022-02-15)
Supplement: Supplementary file 2 [file inner_outer.tex]

\section{Multi-label Conformal Prediction}
\label{app:inner_outer}

Describe \citet{cauchois2020knowing}
